# Supplementary material for: pi-Net: Empirical Latent Representations for Differentiable Physics Heads in Data-Scarce Systems
Source: arXiv:2610.16504 source file (2026-10-12)
Supplement: Supplementary file 1 [file appendix.tex]

\appendix

\section{Additional Experimental Results and Performance Analysis}
\subsection{Confidence Intervals and Statistical Distribution}
To rigorously quantify the generalizability and robustness of the proposed $\pi$-Net framework against purely data-driven baselines, model performance was evaluated across stratified cross-validation folds using three independent random seeds ($1, 42, 123$). Table \ref{tab:ci_performance} summarizes the bootstrap $95\%$ confidence intervals for $R^2$ computed from 1,000 resamples.

\begin{table}[htbp]
    \centering
    \caption{Bootstrap $95\%$ confidence intervals for $R^2$ comparing backbone architectures and their $\pi$-Net variants.}
    \label{tab:ci_performance}
    \begin{tabular}{lcc}
        \toprule
        \textbf{Model} & \textbf{Baseline $R^2$ 95\% CI} & \textbf{$\pi$-Net $R^2$ 95\% CI} \\
        \midrule
        LASSO          & [0.685, 0.789]                 & [0.787, 0.882]                 \\
        MLP            & [0.743, 0.867]                 & [0.794, 0.901]                 \\
        FT-Transformer & [0.722, 0.858]                 & [0.818, 0.903]                 \\
        \bottomrule
    \end{tabular}
\end{table}

\subsection{Training Data Robustness Analysis}
To evaluate how structural physics integration compensates for severe data scarcity, models were trained across progressively constrained data splits (from $80\%$ train split down to $50\%$ training data). Figure \ref{fig:training_split_robustness} illustrates the comparative trends in $R^2$ performance (mean $\pm 1$ standard deviation) across these splits.

\begin{figure}[htbp]
    \centering
    % TODO: Replace 'path_to_your_ci_plot.png' with your actual image file name
    \includegraphics[width=0.95\textwidth]{Images/appendix_image.png}
    \caption{Comparison of $R^2$ performance (mean $\pm 1$ standard deviation) between purely data-driven baselines and $\pi$-Net variants (LASSO, MLP, FT-Transformer) under varying training data-scarcity regimes.}
    \label{fig:training_split_robustness}
\end{figure}

\section{Reproducibility resources}

\subsection{1. Code and Dataset Access}
The complete implementation, architecture source files, baseline comparisons, and the custom $N=60$ robotic Gas Metal Arc Welding (GMAW) experimental dataset are publicly available in the open-source GitHub repository:
\begin{center}
    \url{https://anonymous.4open.science/r/pi-net_repo-4198/README.md}
\end{center}
The repository includes the raw and preprocessed data files (`data_set_updated.csv` / `.xlsx`), the $\pi$-Net framework implementation script, and the pure data-driven baseline scripts.

\subsection{2. Hyperparameters Used}
All models were trained using standard stratified cross-validation protocols. The specific hyperparameters extracted directly from the codebase are detailed below:
\begin{itemize}
    \item \textbf{General Training Settings:} Maximum epochs set to $3000$, early stopping patience of $500$ epochs, batch size of $8$, and gradient clipping threshold at max norm $1.0$.
    \item \textbf{Optimizer & Scheduler:} AdamW optimizer with weight decay of $2 \times 10^{-4}$. Learning rate scheduler uses Cosine Annealing with Warm Restarts ($T_0 = 50$, $T_{mult} = 2$, $\eta_{min} = 1 \times 10^{-6}$).
    \item \textbf{Backbone-Specific Learning Rates:} For the FT-Transformer variants, backbone parameters use a learning rate of $8 \times 10^{-4}$ while the physical output layer ($\pi$ parameters) uses $1.5 \times 10^{-3}$. LASSO variants use a learning rate of $1.5 \times 10^{-3}$ with an L1 regularization alpha of $1 \times 10^{-3}$.
    \item \textbf{LightGBM Settings (when applicable):} Learning rate of $0.05$, $1000$ boosting rounds, early stopping patience of $100$ rounds, $5$ num leaves, and a minimum data in leaf of $3$.
    \item \textbf{Inverse Optimization Parameters:} $2000$ optimization steps per restart, learning rate of $0.01$, $5$ random restarts, and regularization weight $\lambda = 0.2$ to maintain proximity to the regime center.
\end{itemize}

\subsection{3. Compute Resources}
All training, cross-validation evaluation were executed locally on a development laptop with the following specifications:
\begin{itemize}
    \item \textbf{Processor (CPU):} AMD Ryzen 9 8945H with Radeon 780M Graphics (4.00 GHz).
    \item \textbf{Memory (RAM):} 16.0 GB (15.3 GB usable).
    \item \textbf{Graphics Card (GPU):} NVIDIA GeForce RTX 4060 Laptop GPU (8 GB VRAM).
    \item \textbf{Operating System:} 64-bit Windows, x64-based processor.
\end{itemize}
